# Supplementary material for: PyTorch-IE: Fast and Reproducible Prototyping for Information Extraction
Source: arXiv:2406.00007 source file (2024-05-16)
Supplement: Supplementary file 1 [file 99_appendix.tex]

\appendix

\section{Example Appendix}
\label{sec:appendix}

This is an appendix.

\subsection{Document Types}
